# Supplementary material for: Safeguarding E-Commerce against Advisor Cheating Behaviors: Towards More Robust Trust Models for Handling Unfair Ratings
Source: arXiv:1306.4999 source file (2013-06-20)
Supplement: Supplementary file 2 [file appendix2.tex]

\chapter{Appdx B}

and here I put some more postamble ...

% ------------------------------------------------------------------------

%%% Local Variables: 
%%% mode: latex
%%% TeX-master: "../thesis"
%%% End: 
